# Supplementary material for: First Search for Dark Sector $e^+e^-$ Explanations of the MiniBooNE Anomaly at MicroBooNE
Source: arXiv:2502.10900 ancillary file (2025-02-15)
Supplement: Supplementary file 1 [file Supplemental_materials_DarkNeutrino_uBooNE_2025.pdf]

## SUPPLEMENTAL MATERIAL

### Background rich Sidebands

Prior to unblinding the signal region, sidebands adjacent to the signal region rich in both (a) signal-like NC $\pi^0$ and (b) neutrino induced backgrounds where the interaction takes place outside the TPC but resulting daughter particles move inside were studied to ensure that these crucial backgrounds were in agreement with our modeling within assigned uncertainties. The samples are defined as follows;

- (a) This sideband selects events which are more likely to be NC $\pi^0$ by placing a cut on the NC $\pi^0$ rejection BDT of $< 0.8$. This is in conjunction with additional requirements that the cosmic rejection BDT, CC $\nu_\mu$ rejection BDT, and CC $\nu_e$ rejection BDT's are higher than 0.95, 0.9 and 0.2 respectively in order to reduce non- NC $\pi^0$ backgrounds.

- (b) This sideband is defined as all events where the distance backwards along the primary shower direction from the reconstructed shower start to the nearest TPC wall is $<$ 50cm, in conjunction with a cosmic rejection BDT cut of $> 0.9$.

Both samples are fully statistically independent selections to the final selected signal samples and in both cases less than 5 signal events would be expected for signals consistent with the MiniBooNE anomaly. In all the variables studied we saw good agreement in these sidebands, building confidence in our background predictions. See Fig. 1 for two representative examples of these sidebands studies, with $\chi^2/\mathrm{n}d.o.f.$ values of 14.11/22 and 9.78/20 highlighting the observed agreement.

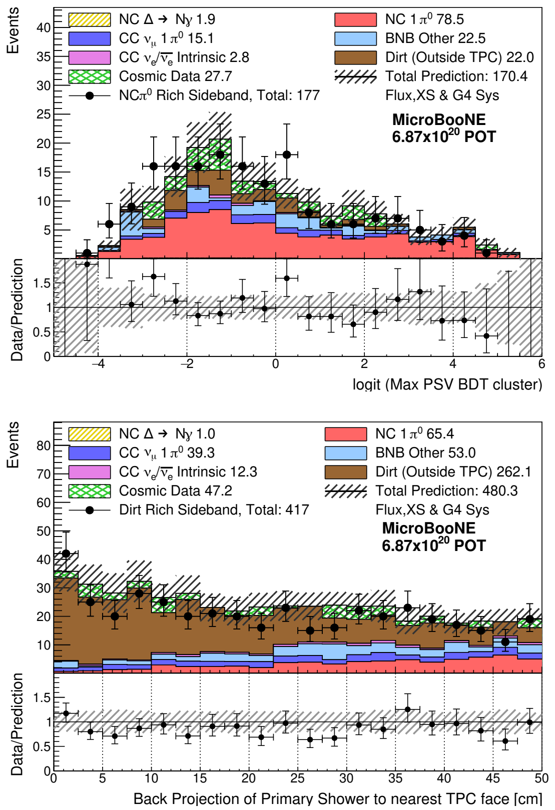


FIG. 1. *Top*: The NC $\pi^0$ rich sideband developed to study the cluster based variables such as the proton stub veto BDT score, as described in [1]. *Bottom*: Sideband rich in events scattering into the TPC from outside, showing the distance between the highest energy reconstructed shower and nearest TPC face following along the backward projection of the shower direction. Events containing showers that scatter into the TPC from outside tend to cluster up with backward projections closer to zero. In both sidebands, good agreement was found within assigned uncertainty. These plots have flux, interaction and Geant4 systematic uncertainties included but do not include detector systematics.

### Constraining NC $\pi^0$ Two-Shower Sidebands

Figure 2 shows the two high-statistics two-shower NC $\pi^0$ selections used to constrain the large NC $\pi^0$ cross-section uncertainties associated with the primary backgrounds to our $e^+e^-$ signals. These two samples are defined by taking the full two-shower NC $\pi^0$ sample and splitting it based on the number of observed reconstructed proton tracks. The threshold for detecting such protons is approximately 50 MeV true proton kinetic energy. These are very similar to prior NC $\pi^0$ samples used for constraints in [2] and for cross-section measurements in [3] but with a minor increase in data POT from $5.89 \times 10^{20}$ to $6.87 \times 10^{20}$ due to reprocessing and an improved cosmic rejection capability due to a retraining of the cosmic rejection BDT with higher statistics leading to an increased purity especially in the $2\gamma 0p$ channel.

### Simulation of Scattering in Soil and Clay Preceding Detector

For long-lived dark neutrinos, the simulation of the soil and clay preceding the detector is important to include because a sizable number of observable signal events may be produced in neutrino interactions outside of the detector, eventually entering and decaying in the TPC volume. In addition to the standard BNB flux and detector systematics, an additional 7.87% systematic uncertainty is included on the dark neutrino signal sample to cover any potential discrepancies due to how this scattering is modeled in DarkNews. This uncertainty is dominated by a 7.0% uncertainty on the density of the soil/clay itself including taking into account the varied water content of the soil. In theory, a flat density shift should

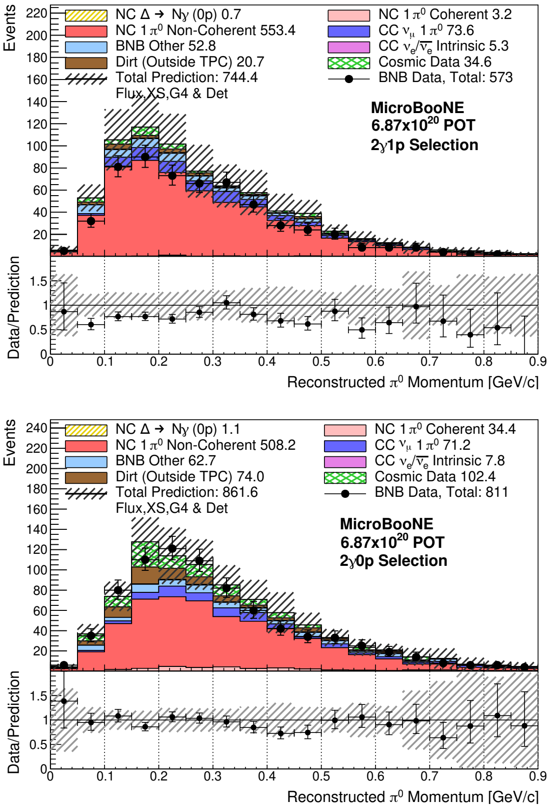


FIG. 2. *Top (Bottom)*: the $2\gamma 1p$ ($2\gamma 0p$) NC $\pi^0$ rich selections used to constrain the NC $\pi^0$ backgrounds during the fitting procedure.

be correlated between bins. However as different regions of varying density could give rise to different energies of signal, we treat the uncertainties as bin-to-bin uncorrelated to be conservative. Subleading effects that are also included are spectral distortions expected when scaling the MicroBooNE flux from the TPC face backward by $1/R^2$ (3.0%), uncertainty on parent meson decay position (1.3%), and uncertainty on mineral content in the soil composition (modeled as $SiO_2$ in DarkNews, 1.5%).

### Additional Efficiency Information

There is large interplay between the efficiency of the selection and the four key kinematic variables of the dark sector signals, total $e^+e^-$ energy, the angle the $e^+e^-$ makes with respect to the beam, the $e^+e^-$ energy asymmetry (defined as $|E_{e^+} - E_{e^-}|/(E_{e^+} - E_{e^-})$), and the $e^+e^-$ opening angle. This is even more true when one considers the three reconstructible topologies that this analysis targets, the single-shower, two-shower , and one-shower plus one-track. Figure 3 highlights this effect showing that for low $e^+e^-$ opening angles the single-shower topology dominates but for larger values the contributions from the two other topologies become comparable. Shown also for completeness is the efficiency as a function of the final two kinematic variables, true $e^+e^-$ energy asymmetry, in the same style as Fig. ??.

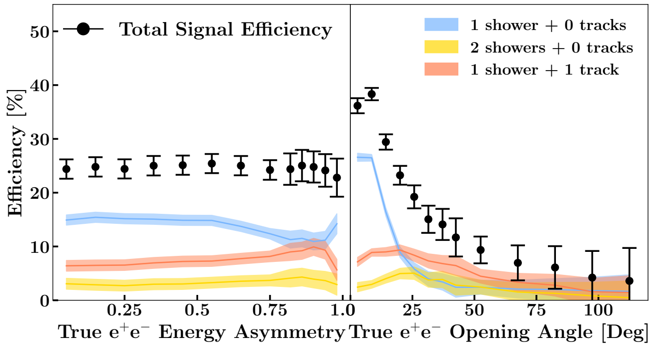


FIG. 3. Signal efficiency as a function of (a) true $e^+e^-$ opening angle and (b) true $e^+e^-$ energy asymmetry. Shown also is the split in efficiency between the three topologies that this analysis targets.

### Pre-Constraint Final Selection Events

Figure 4 shows the same three final selection distributions as in Fig. ?? but prior to NC $\pi^0$ constraint and with a breakdown of expected background categories. Without the constraint we have a slightly higher background rate and, also, larger uncertainties, but the observed data is still in good agreement with the predictions with $\chi^2/nd.o.f.$ values of 1.08/6, 6.93/5, and 0.84/4 for total reconstructed visible energy, reconstructed primary shower angle and NC $\pi^0$ BDT score respectively.

### Model Assumptions

We now state the model assumptions in this analysis in more detail. In dual dark neutrino models, the scattering of low-energy flavor states $|\nu_\mu\rangle = \sum_{i=1}^{3} U_{\mu i} |\nu_i\rangle$ produced in pion and kaon decays into a dark neutrino mass eigenstate $\nu_4$ or $\nu_5$ in the detector is proportional to

$$V_{\mu h} \equiv U_{Dh} \frac{U_{\mu 4} U_{D4}^* + U_{\mu 5} U_{D5}^*}{\sqrt{1 - \sum_{\alpha=e}^{\tau} (|U_{\alpha 4}|^2 + |U_{\beta 5}|^2)}}. \quad (1)$$

Here, $U_{Dh}$ stands for the mixing element between the dark flavor states (collectively denoted by $\nu_D$) and the mass eigenstate $\nu_h \in \{\nu_4, \nu_5\}$. For a single dark neutrino models, analogous expressions hold with $U_{\alpha 5} = 0$. This analysis assumes that $|U_{\mu 4}| = |U_{\mu 5}|$ and $|U_{D4}| = |U_{D5}|$.

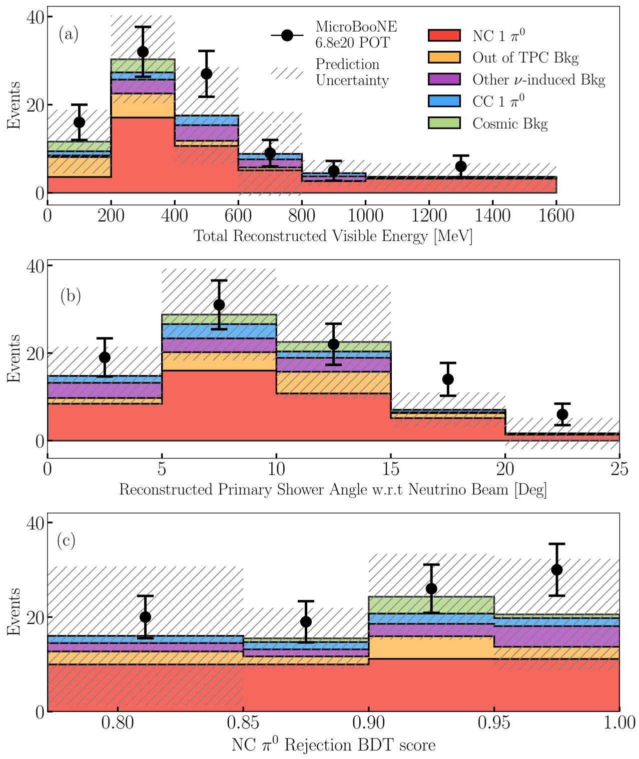


FIG. 4. Final selected data and simulation prediction for the $e^+e^-$ signal region. Shown are the total reconstructed visible energy (a), the angle the primary reconstructed shower makes with respect to the incoming neutrino beam (b), and the NC $\pi^0$ BDT rejection score (c). In all cases we see good agreement between observed data and our background-only predictions with $\chi^2/\mathrm{n}.d.o.f.$ of respectively.

Therefore, taking $|U_{D4}|^2 = |U_{D5}|^2 = 1/2$, we conclude that $|V_{\mu 4(5)}| = |U_{\mu 4(5)}|$, the latter being a more familiar parameter from the literature in heavy neutral leptons and what is used in this letter. Similarly, in the decay of a dark neutrino to light mass eigenstates, the combination of mixing parameters becomes proportional to the small parameter $\sum_\alpha |U_{\alpha 4}|^2$ and in the decay $\nu_5 \to \nu_4 e^+e^-$ it becomes proportional to $|U_{D5}U_{D4}|^2 = 1/4$. The exact interdependence of the mixing elements is highly model dependent, so our choices are justified by their simplicity. The dark neutrinos are assumed to be Dirac particles. The kinematics in the case of Majorana dark neutrinos is somewhat different but is also less compatible with the MiniBooNE event distributions.


[1] P. Abratenko *et al.* (MicroBooNE), First search for neutral current coherent single-photon production in microboone (2025), arXiv:2502.06091 [hep-ex].

[2] P. Abratenko *et al.* (MicroBooNE), Search for Neutrino-Induced Neutral-Current Δ Radiative Decay in MicroBooNE and a First Test of the MiniBooNE Low Energy Excess under a Single-Photon Hypothesis, Phys. Rev. Lett. **128**, 111801 (2022), arXiv:2110.00409 [hep-ex].

[3] P. Abratenko *et al.* (MicroBooNE), Measurement of neutral current single π0 production on argon with the MicroBooNE detector, Phys. Rev. D **107**, 012004 (2023), arXiv:2205.07943 [hep-ex].
